# Supplementary material for: Client-side Gradient Inversion Against Federated Learning from Poisoning
Source: arXiv:2309.07415 source file (2023-09-14)
Supplement: Supplementary file 1 [file appendix.tex]

% \onecolumn
\section{Additional Result}
\begin{table*}[h]
\caption{CTGI Inversion Result based on threat models. These results are produced under the condition that threat models can totally replace the global model. Inversion images reflect the inversion ability of threat models.}
\label{Table_InversionResult2}

\begin{subtable}{\linewidth}
\centering
\resizebox{\linewidth}{!}{
\fontsize{30pt}{20pt}\selectfont
\begin{tblr}{
  width = \linewidth,
  cells = {c},
  cell{1}{2} = {c=4}{},
  cell{1}{6} = {c=4}{},
  cell{1}{10} = {c=4}{},
  vline{2-3,7} = {1}{},
  vline{2,6,10} = {2-8}{},
  hline{4,6} = {-}{},
}
Threat Model & Model Retrain (MR) &         &          &          & Model Poisoning (MP) &         &         &         & Model Inversion
  Poisoning (MIP) &         &          &          \\
AGR          & M-Krum          & Bulyan  & AFA      & Fang     & M-Krum            & Bulyan  & AFA     & Fang    & M-Krum                         & Bulyan  & AFA      & Fang     \\
Setting      & 32x50 10           & 32x50 9 & 32x50 10 & 32x50 10 & 32x40 8              & 32x40 7 & 32x40 8 & 32x40 8 & 32x50 10                        & 32x50 9 & 32x50 10 & 32x50 10 \\
Original     &\SetCell[r=1]{l}{\begin{minipage}[b]{0.25\columnwidth}
		\raisebox{-.5\height}{\includegraphics[width=1.0\linewidth]{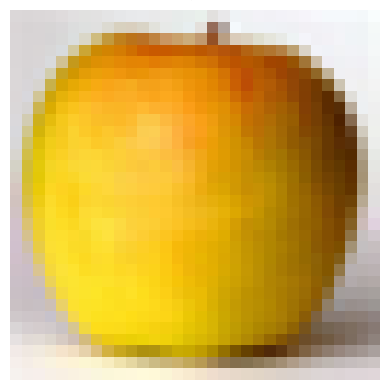}}
	\end{minipage}}      
            & \SetCell[r=1]{l}{\begin{minipage}[b]{0.25\columnwidth}
		\raisebox{-.5\height}{\includegraphics[width=1.0\linewidth]{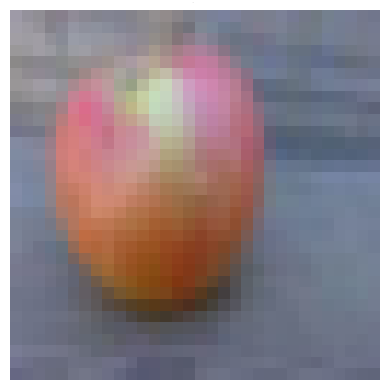}}
	\end{minipage}}         
            & \SetCell[r=1]{l}{\begin{minipage}[b]{0.25\columnwidth}
		\raisebox{-.5\height}{\includegraphics[width=1.0\linewidth]{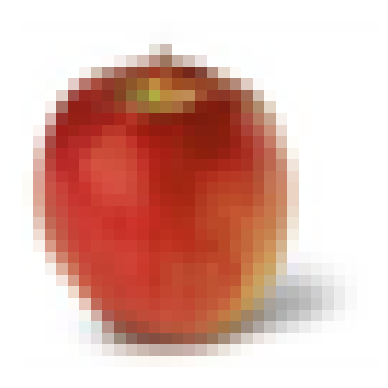}}
	\end{minipage}}  
            & \SetCell[r=1]{l}{\begin{minipage}[b]{0.25\columnwidth}
		\raisebox{-.5\height}{\includegraphics[width=1.0\linewidth]{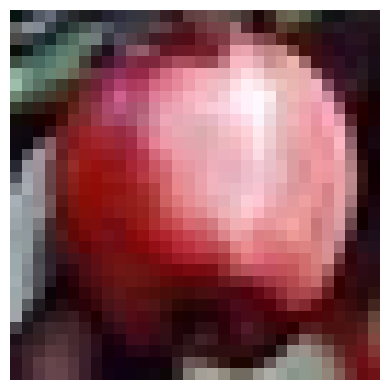}}
	\end{minipage}}  
            & \SetCell[r=1]{l}{\begin{minipage}[b]{0.25\columnwidth}
		\raisebox{-.5\height}{\includegraphics[width=1.0\linewidth]{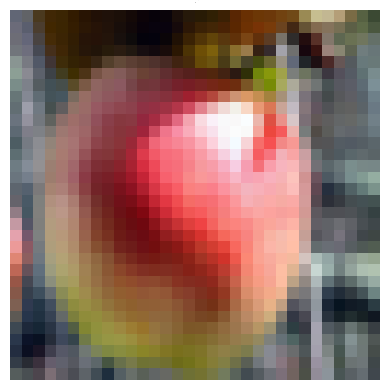}}
	\end{minipage}}                      
            & \SetCell[r=1]{l}{\begin{minipage}[b]{0.25\columnwidth}
		\raisebox{-.5\height}{\includegraphics[width=1.0\linewidth]{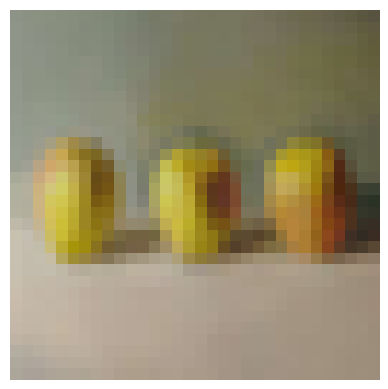}}
	\end{minipage}}  
            & \SetCell[r=1]{l}{\begin{minipage}[b]{0.25\columnwidth}
		\raisebox{-.5\height}{\includegraphics[width=1.0\linewidth]{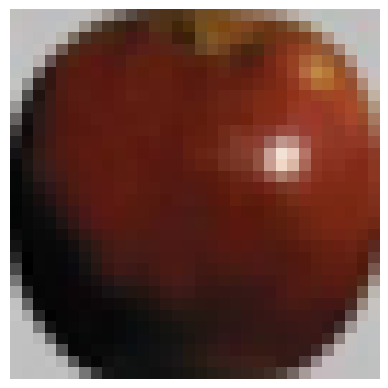}}
	\end{minipage}}  
            & \SetCell[r=1]{l}{\begin{minipage}[b]{0.25\columnwidth}
		\raisebox{-.5\height}{\includegraphics[width=1.0\linewidth]{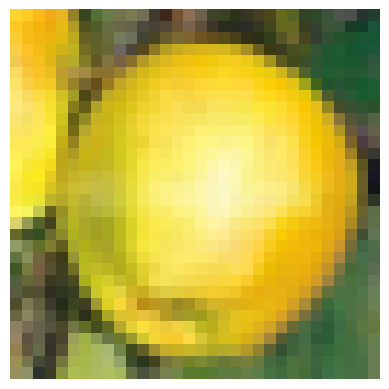}}
	\end{minipage}}
            & \SetCell[r=1]{l}{\begin{minipage}[b]{0.25\columnwidth}
		\raisebox{-.5\height}{\includegraphics[width=1.0\linewidth]{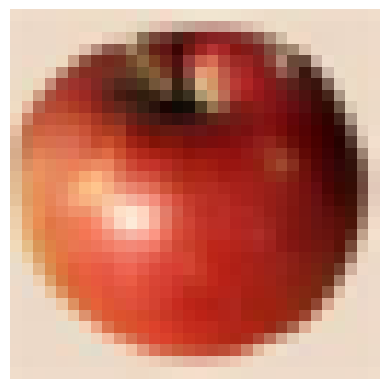}}
	\end{minipage}}
            & \SetCell[r=1]{l}{\begin{minipage}[b]{0.25\columnwidth}
		\raisebox{-.5\height}{\includegraphics[width=1.0\linewidth]{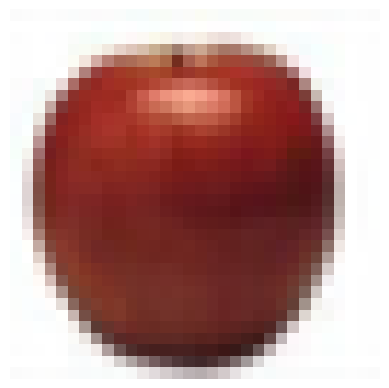}}
	\end{minipage}}
            & \SetCell[r=1]{l}{\begin{minipage}[b]{0.25\columnwidth}
		\raisebox{-.5\height}{\includegraphics[width=1.0\linewidth]{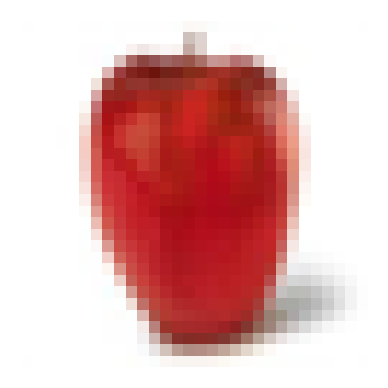}}
	\end{minipage}}
            & \SetCell[r=1]{l}{\begin{minipage}[b]{0.25\columnwidth}
		\raisebox{-.5\height}{\includegraphics[width=1.0\linewidth]{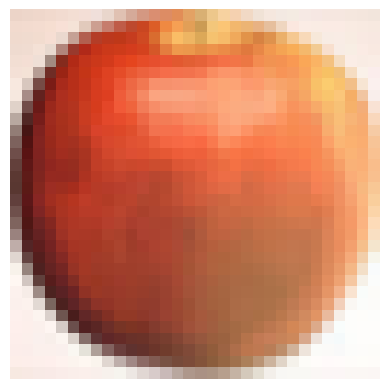}}
	\end{minipage}}
            \\
Inverse    &\SetCell[r=1]{l}{\begin{minipage}[b]{0.25\columnwidth}
		\raisebox{-.5\height}{\includegraphics[width=1.0\linewidth]{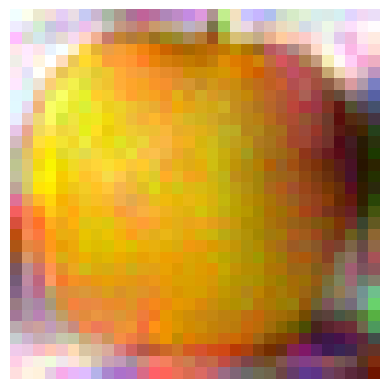}}
	\end{minipage}}      
            & \SetCell[r=1]{l}{\begin{minipage}[b]{0.25\columnwidth}
		\raisebox{-.5\height}{\includegraphics[width=1.0\linewidth]{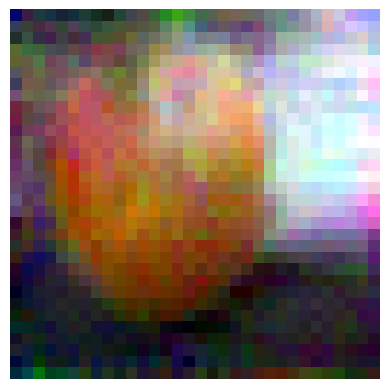}}
	\end{minipage}}         
            & \SetCell[r=1]{l}{\begin{minipage}[b]{0.25\columnwidth}
		\raisebox{-.5\height}{\includegraphics[width=1.0\linewidth]{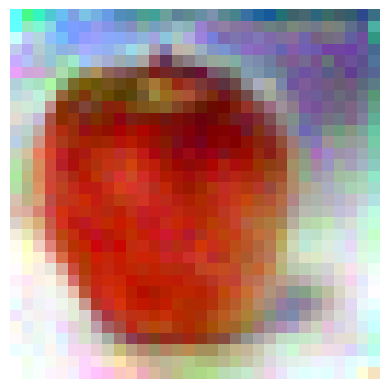}}
	\end{minipage}}  
            & \SetCell[r=1]{l}{\begin{minipage}[b]{0.25\columnwidth}
		\raisebox{-.5\height}{\includegraphics[width=1.0\linewidth]{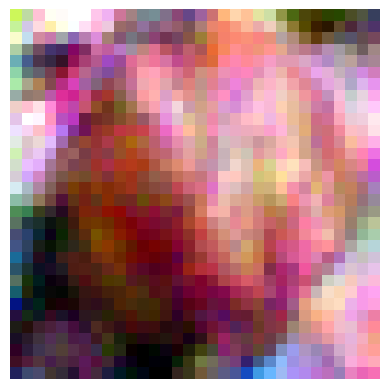}}
	\end{minipage}}  
            & \SetCell[r=1]{l}{\begin{minipage}[b]{0.25\columnwidth}
		\raisebox{-.5\height}{\includegraphics[width=1.0\linewidth]{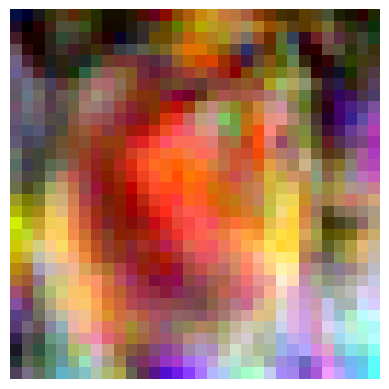}}
	\end{minipage}}                      
            & \SetCell[r=1]{l}{\begin{minipage}[b]{0.25\columnwidth}
		\raisebox{-.5\height}{\includegraphics[width=1.0\linewidth]{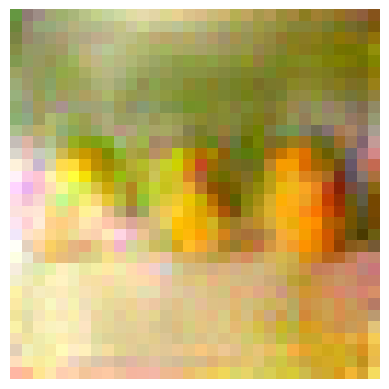}}
	\end{minipage}}  
            & \SetCell[r=1]{l}{\begin{minipage}[b]{0.25\columnwidth}
		\raisebox{-.5\height}{\includegraphics[width=1.0\linewidth]{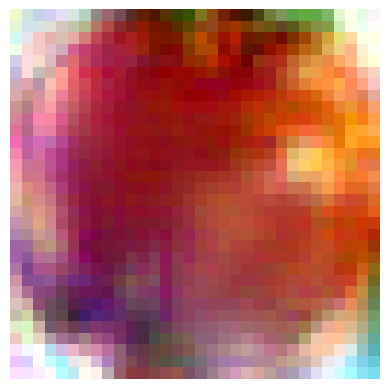}}
	\end{minipage}}  
            & \SetCell[r=1]{l}{\begin{minipage}[b]{0.25\columnwidth}
		\raisebox{-.5\height}{\includegraphics[width=1.0\linewidth]{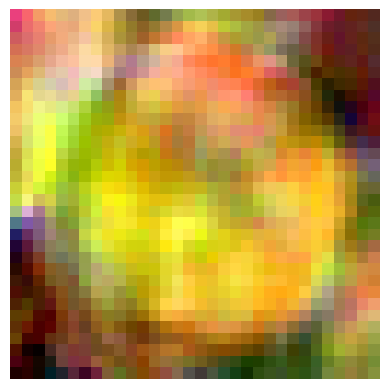}}
	\end{minipage}}
            & \SetCell[r=1]{l}{\begin{minipage}[b]{0.25\columnwidth}
		\raisebox{-.5\height}{\includegraphics[width=1.0\linewidth]{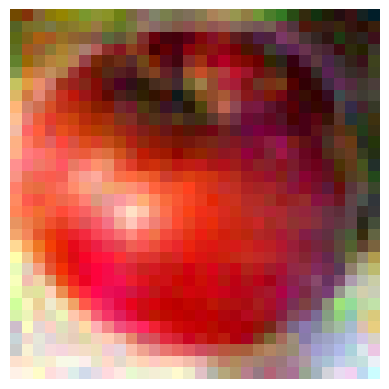}}
	\end{minipage}}
            & \SetCell[r=1]{l}{\begin{minipage}[b]{0.25\columnwidth}
		\raisebox{-.5\height}{\includegraphics[width=1.0\linewidth]{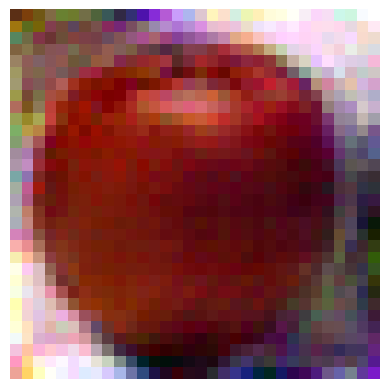}}
	\end{minipage}}
            & \SetCell[r=1]{l}{\begin{minipage}[b]{0.25\columnwidth}
		\raisebox{-.5\height}{\includegraphics[width=1.0\linewidth]{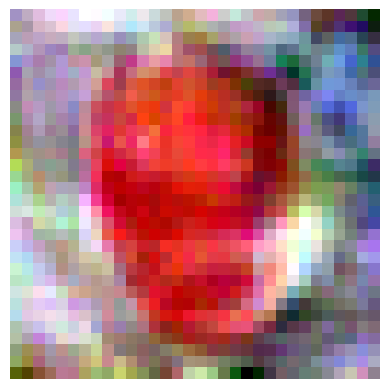}}
	\end{minipage}}
            & \SetCell[r=1]{l}{\begin{minipage}[b]{0.25\columnwidth}
		\raisebox{-.5\height}{\includegraphics[width=1.0\linewidth]{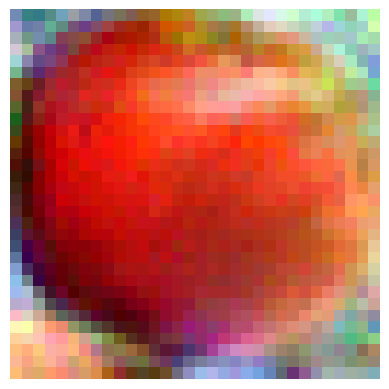}}
	\end{minipage}}     
            \\
PSNR        & 14.729 & 11.230 & 11.739 &	10.260 & 12.397 & 15.187 & 10.810 & 13.100	12.258 & 9.588 & 8.885 & 14.048
   \\
LPIPS        & 0.205 & 0.265 & 0.145 &	0.491 & 0.463 & 0.418 & 0.42 & 0.535	0.166 & 0.173 & 0.412 & 0.221
    \\
SSIM         & 0.503 & 0.35 & 0.601 & 0.331	& 0.474	& 0.473 & 0.279 & 0.174 & 0.578	0.582 & 0.318 & 0.488
    
\end{tblr}
}
\caption{CTGI inversion result on Cifar100}
\label{SubTable_appInversionResultSubCifar}
\end{subtable}

\begin{subtable}{\linewidth}
\centering
\resizebox{\linewidth}{!}{
\fontsize{30pt}{20pt}\selectfont
\begin{tblr}{
  width = \linewidth,
  cells = {c},
  cell{1}{2} = {c=4}{},
  cell{1}{6} = {c=4}{},
  cell{1}{10} = {c=4}{},
  vline{2-3,7} = {1}{},
  vline{2,6,10} = {2-8}{},
  hline{4,6} = {-}{},
}
Threat Model & Model Retrain (MR) &         &          &          & Model Poisoning (MP) &         &         &         & Model Inversion
  Poisoning (MIP) &         &          &          \\
AGR          & M-Krum          & Bulyan  & AFA      & Fang     & M-Krum            & Bulyan  & AFA     & Fang    & M-Krum                         & Bulyan  & AFA      & Fang     \\
Setting      & 32x40 8            & 32x40 7  & 32x40 8  & 32x40 8  & 32x30 6              & 32x30 5 & 32x30 6 & 32x30 6 & 32x40 8                         & 32x40 7  & 32x40 8  & 32x40 8  \\
Original     &\SetCell[r=1]{l}{\begin{minipage}[b]{0.25\columnwidth}
		\raisebox{-.5\height}{\includegraphics[width=1.0\linewidth]{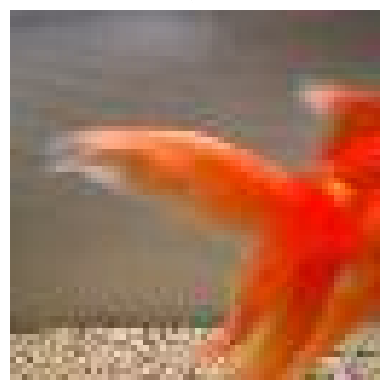}}
	\end{minipage}}      
            & \SetCell[r=1]{l}{\begin{minipage}[b]{0.25\columnwidth}
		\raisebox{-.5\height}{\includegraphics[width=1.0\linewidth]{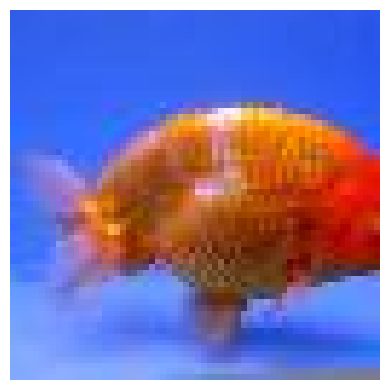}}
	\end{minipage}}         
            & \SetCell[r=1]{l}{\begin{minipage}[b]{0.25\columnwidth}
		\raisebox{-.5\height}{\includegraphics[width=1.0\linewidth]{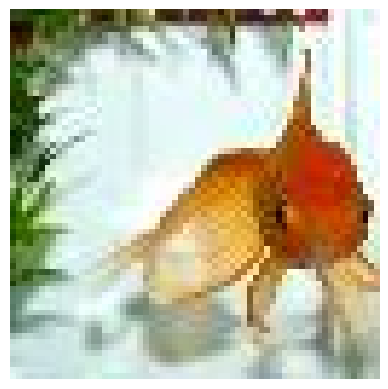}}
	\end{minipage}}  
            & \SetCell[r=1]{l}{\begin{minipage}[b]{0.25\columnwidth}
		\raisebox{-.5\height}{\includegraphics[width=1.0\linewidth]{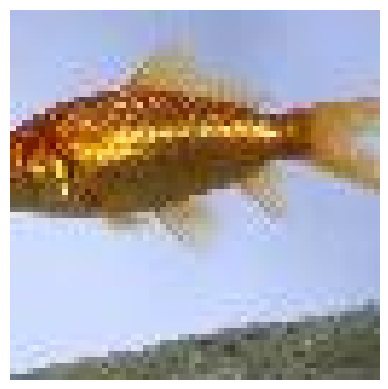}}
	\end{minipage}}  
            & \SetCell[r=1]{l}{\begin{minipage}[b]{0.25\columnwidth}
		\raisebox{-.5\height}{\includegraphics[width=1.0\linewidth]{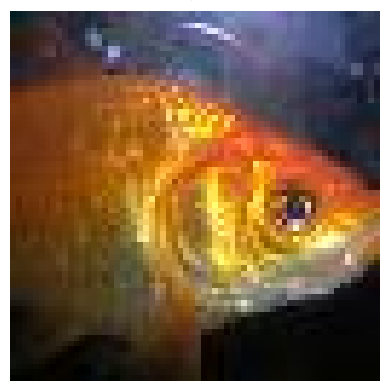}}
	\end{minipage}}                      
            & \SetCell[r=1]{l}{\begin{minipage}[b]{0.25\columnwidth}
		\raisebox{-.5\height}{\includegraphics[width=1.0\linewidth]{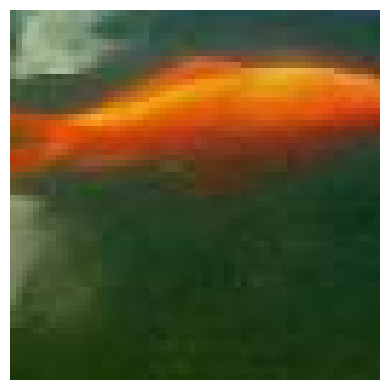}}
	\end{minipage}}  
            & \SetCell[r=1]{l}{\begin{minipage}[b]{0.25\columnwidth}
		\raisebox{-.5\height}{\includegraphics[width=1.0\linewidth]{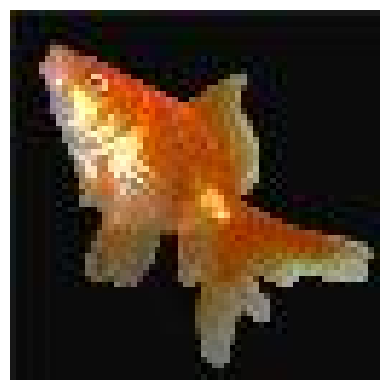}}
	\end{minipage}}  
            & \SetCell[r=1]{l}{\begin{minipage}[b]{0.25\columnwidth}
		\raisebox{-.5\height}{\includegraphics[width=1.0\linewidth]{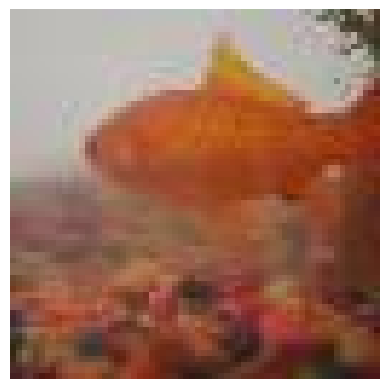}}
	\end{minipage}}
            & \SetCell[r=1]{l}{\begin{minipage}[b]{0.25\columnwidth}
		\raisebox{-.5\height}{\includegraphics[width=1.0\linewidth]{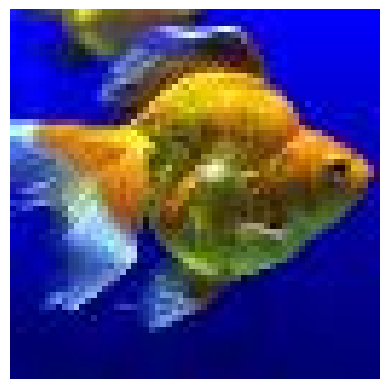}}
	\end{minipage}}
            & \SetCell[r=1]{l}{\begin{minipage}[b]{0.25\columnwidth}
		\raisebox{-.5\height}{\includegraphics[width=1.0\linewidth]{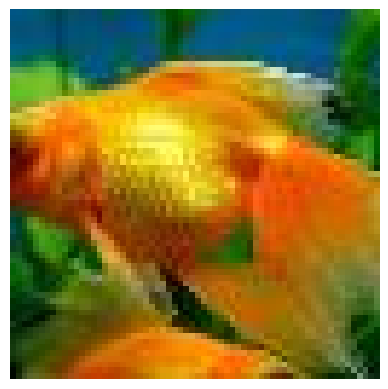}}
	\end{minipage}}
            & \SetCell[r=1]{l}{\begin{minipage}[b]{0.25\columnwidth}
		\raisebox{-.5\height}{\includegraphics[width=1.0\linewidth]{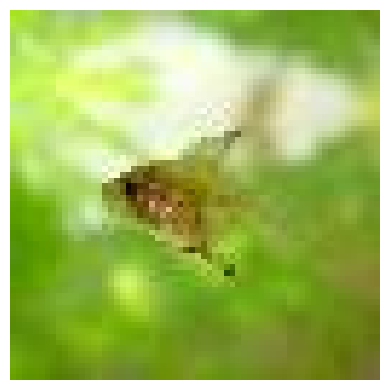}}
	\end{minipage}}
            & \SetCell[r=1]{l}{\begin{minipage}[b]{0.25\columnwidth}
		\raisebox{-.5\height}{\includegraphics[width=1.0\linewidth]{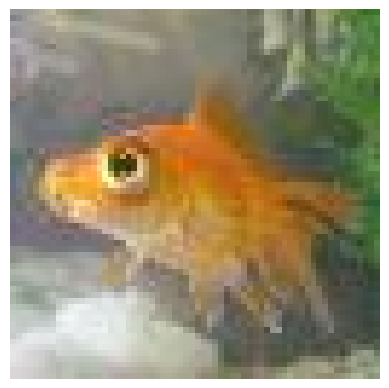}}
	\end{minipage}}
            \\
Inverse    &\SetCell[r=1]{l}{\begin{minipage}[b]{0.25\columnwidth}
		\raisebox{-.5\height}{\includegraphics[width=1.0\linewidth]{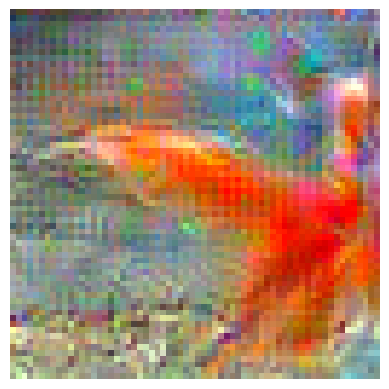}}
	\end{minipage}}      
            & \SetCell[r=1]{l}{\begin{minipage}[b]{0.25\columnwidth}
		\raisebox{-.5\height}{\includegraphics[width=1.0\linewidth]{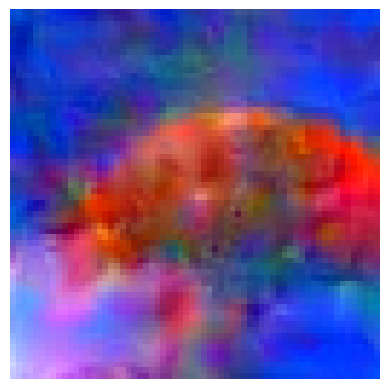}}
	\end{minipage}}         
            & \SetCell[r=1]{l}{\begin{minipage}[b]{0.25\columnwidth}
		\raisebox{-.5\height}{\includegraphics[width=1.0\linewidth]{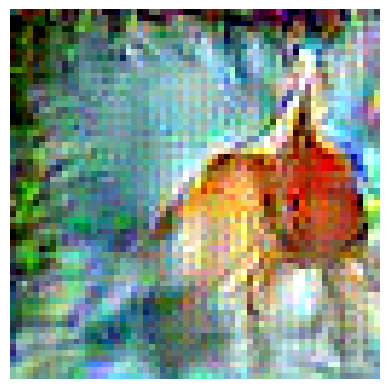}}
	\end{minipage}}  
            & \SetCell[r=1]{l}{\begin{minipage}[b]{0.25\columnwidth}
		\raisebox{-.5\height}{\includegraphics[width=1.0\linewidth]{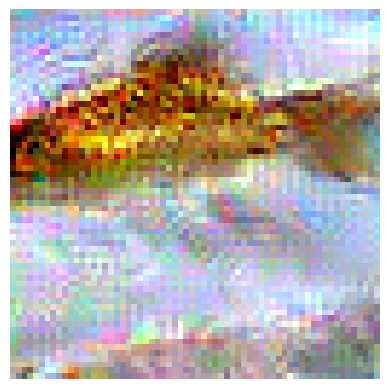}}
	\end{minipage}}  
            & \SetCell[r=1]{l}{\begin{minipage}[b]{0.25\columnwidth}
		\raisebox{-.5\height}{\includegraphics[width=1.0\linewidth]{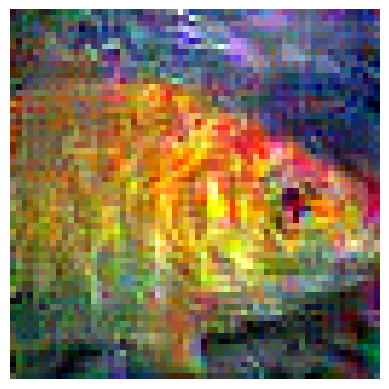}}
	\end{minipage}}                      
            & \SetCell[r=1]{l}{\begin{minipage}[b]{0.25\columnwidth}
		\raisebox{-.5\height}{\includegraphics[width=1.0\linewidth]{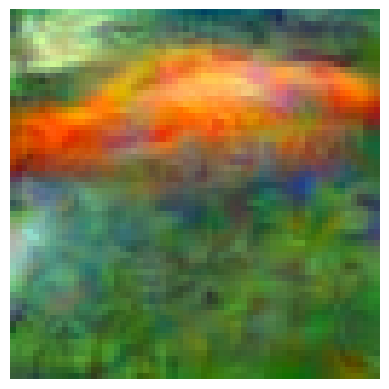}}
	\end{minipage}}  
            & \SetCell[r=1]{l}{\begin{minipage}[b]{0.25\columnwidth}
		\raisebox{-.5\height}{\includegraphics[width=1.0\linewidth]{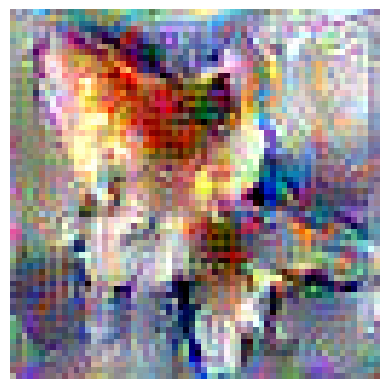}}
	\end{minipage}}  
            & \SetCell[r=1]{l}{\begin{minipage}[b]{0.25\columnwidth}
		\raisebox{-.5\height}{\includegraphics[width=1.0\linewidth]{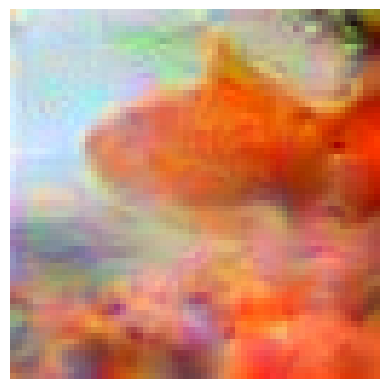}}
	\end{minipage}}
            & \SetCell[r=1]{l}{\begin{minipage}[b]{0.25\columnwidth}
		\raisebox{-.5\height}{\includegraphics[width=1.0\linewidth]{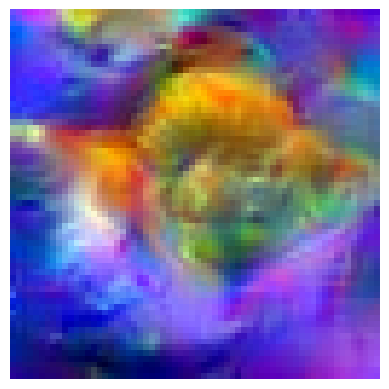}}
	\end{minipage}}
            & \SetCell[r=1]{l}{\begin{minipage}[b]{0.25\columnwidth}
		\raisebox{-.5\height}{\includegraphics[width=1.0\linewidth]{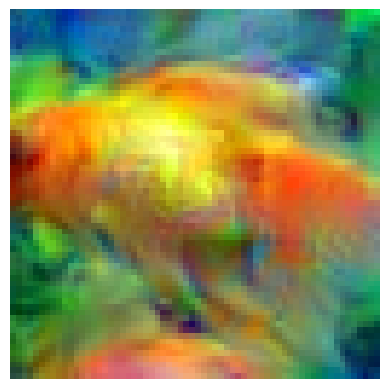}}
	\end{minipage}}
            & \SetCell[r=1]{l}{\begin{minipage}[b]{0.25\columnwidth}
		\raisebox{-.5\height}{\includegraphics[width=1.0\linewidth]{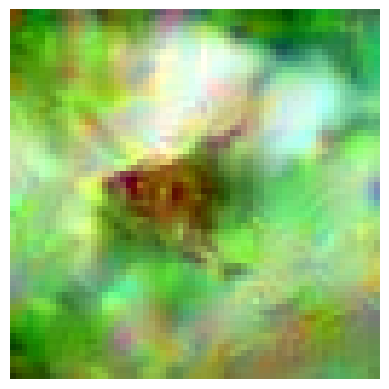}}
	\end{minipage}}
            & \SetCell[r=1]{l}{\begin{minipage}[b]{0.25\columnwidth}
		\raisebox{-.5\height}{\includegraphics[width=1.0\linewidth]{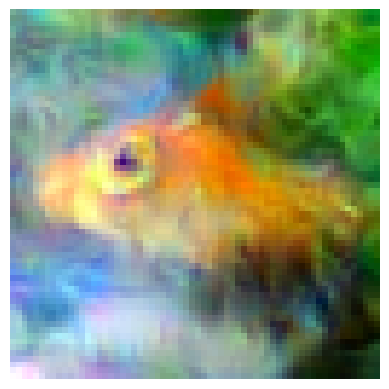}}
	\end{minipage}}     
            \\
PSNR         &15.776&13.785&10.427&14.036&14.830&15.726&6.632&13.550&11.599&15.533&13.916&15.076   \\
LPIPS        &0.418&0.413&0.427&0.475&0.478&0.363&0.575&0.356&0.421&0.255&0.356&0.355    \\
SSIM &0.225&0.340&0.250&0.201&0.203&0.368&0.104&0.409&0.246&0.372&0.365&0.287
\end{tblr}
}
\caption{CTGI inversion result on TinyImageNet }
\label{SubTable_appInversionResultSubImageNet}
\end{subtable}

\begin{subtable}{\linewidth}
\centering
\resizebox{\linewidth}{!}{
\fontsize{30pt}{20pt}\selectfont
\begin{tblr}{
  width = \linewidth,
  cells = {c},
  cell{1}{2} = {c=4}{},
  cell{1}{6} = {c=4}{},
  cell{1}{10} = {c=4}{},
  vline{2-3,7} = {1}{},
  vline{2,6,10} = {2-8}{},
  hline{4,6} = {-}{},
}
Threat Model & Model Retrain (MR) &         &          &          & Model Poisoning (MP) &         &         &         & Model Inversion
  Poisoning (MIP) &         &          &          \\
AGR          & M-Krum          & Bulyan  & AFA      & Fang     & M-Krum            & Bulyan  & AFA     & Fang    & M-Krum                         & Bulyan  & AFA      & Fang     \\
Setting      & 8x10 2             & 8x11 2   & 8x10 2   & 8x10 2   & 8x10 2               & 8x11 2  & 8x10 2  & 8x10 2  & 8x10 2                          & 8x11 2   & 8x10 2   & 8x10 2   \\
Original     &\SetCell[r=1]{l}{\begin{minipage}[b]{0.25\columnwidth}
		\raisebox{-.5\height}{\includegraphics[width=1.0\linewidth]{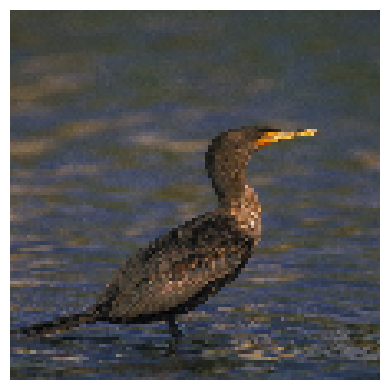}}
	\end{minipage}}      
            & \SetCell[r=1]{l}{\begin{minipage}[b]{0.25\columnwidth}
		\raisebox{-.5\height}{\includegraphics[width=1.0\linewidth]{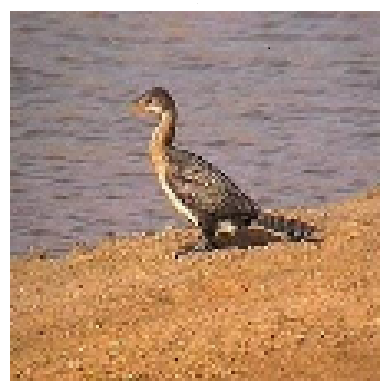}}
	\end{minipage}}         
            & \SetCell[r=1]{l}{\begin{minipage}[b]{0.25\columnwidth}
		\raisebox{-.5\height}{\includegraphics[width=1.0\linewidth]{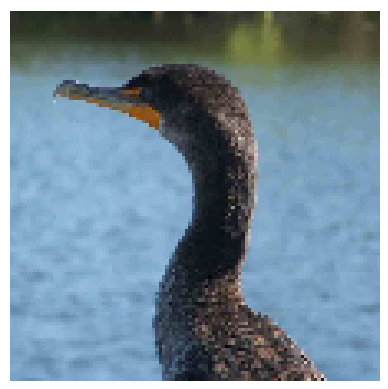}}
	\end{minipage}}  
            & \SetCell[r=1]{l}{\begin{minipage}[b]{0.25\columnwidth}
		\raisebox{-.5\height}{\includegraphics[width=1.0\linewidth]{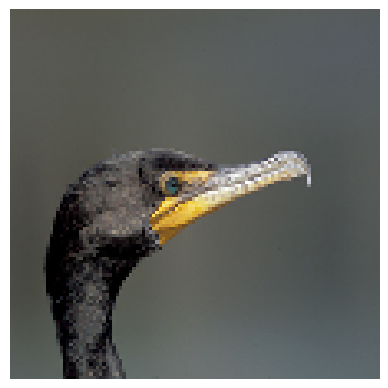}}
	\end{minipage}}  
            & \SetCell[r=1]{l}{\begin{minipage}[b]{0.25\columnwidth}
		\raisebox{-.5\height}{\includegraphics[width=1.0\linewidth]{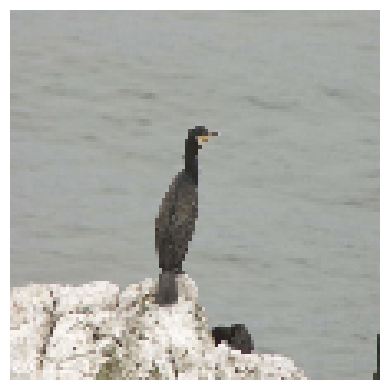}}
	\end{minipage}}                      
            & \SetCell[r=1]{l}{\begin{minipage}[b]{0.25\columnwidth}
		\raisebox{-.5\height}{\includegraphics[width=1.0\linewidth]{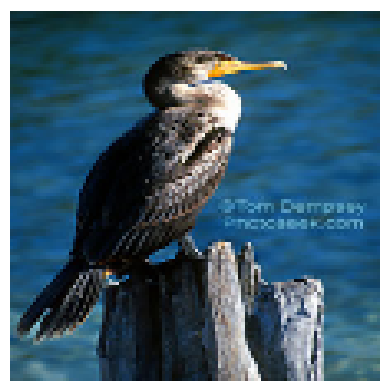}}
	\end{minipage}}  
            & \SetCell[r=1]{l}{\begin{minipage}[b]{0.25\columnwidth}
		\raisebox{-.5\height}{\includegraphics[width=1.0\linewidth]{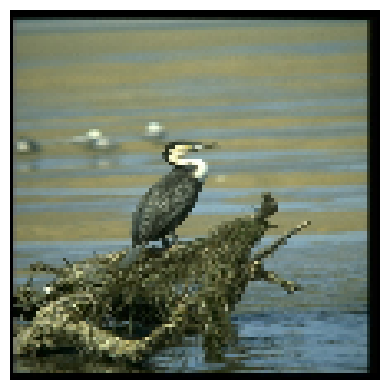}}
	\end{minipage}}  
            & \SetCell[r=1]{l}{\begin{minipage}[b]{0.25\columnwidth}
		\raisebox{-.5\height}{\includegraphics[width=1.0\linewidth]{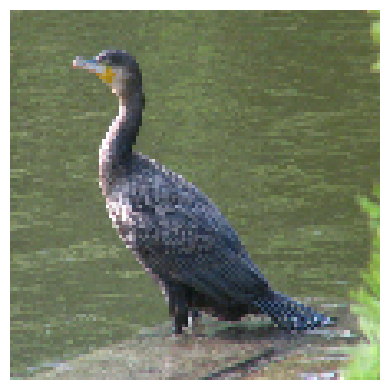}}
	\end{minipage}}
            & \SetCell[r=1]{l}{\begin{minipage}[b]{0.25\columnwidth}
		\raisebox{-.5\height}{\includegraphics[width=1.0\linewidth]{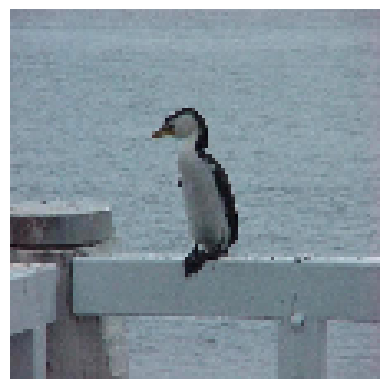}}
	\end{minipage}}
            & \SetCell[r=1]{l}{\begin{minipage}[b]{0.25\columnwidth}
		\raisebox{-.5\height}{\includegraphics[width=1.0\linewidth]{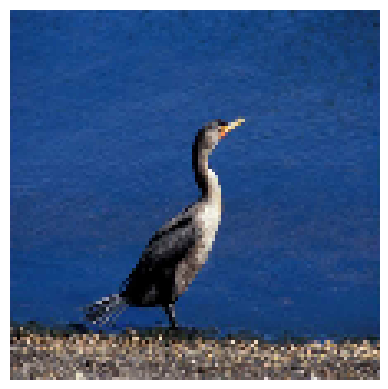}}
	\end{minipage}}
            & \SetCell[r=1]{l}{\begin{minipage}[b]{0.25\columnwidth}
		\raisebox{-.5\height}{\includegraphics[width=1.0\linewidth]{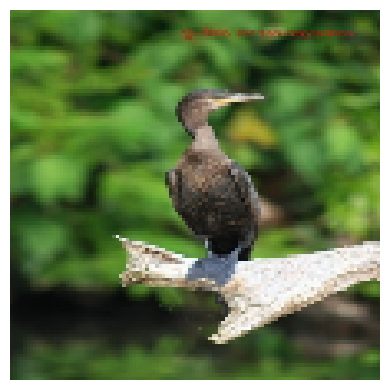}}
	\end{minipage}}
            & \SetCell[r=1]{l}{\begin{minipage}[b]{0.25\columnwidth}
		\raisebox{-.5\height}{\includegraphics[width=1.0\linewidth]{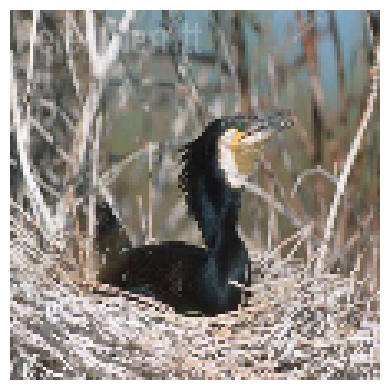}}
	\end{minipage}}
            \\
Inverse    &\SetCell[r=1]{l}{\begin{minipage}[b]{0.25\columnwidth}
		\raisebox{-.5\height}{\includegraphics[width=1.0\linewidth]{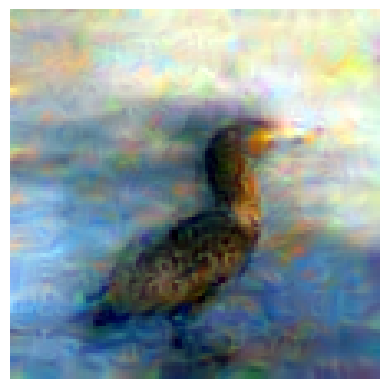}}
	\end{minipage}}      
            & \SetCell[r=1]{l}{\begin{minipage}[b]{0.25\columnwidth}
		\raisebox{-.5\height}{\includegraphics[width=1.0\linewidth]{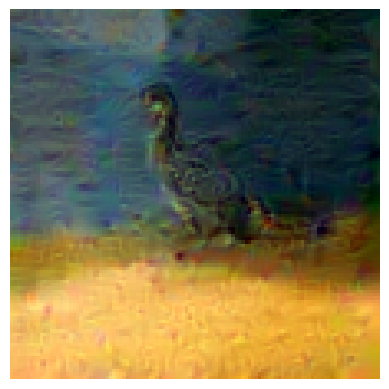}}
	\end{minipage}}         
            & \SetCell[r=1]{l}{\begin{minipage}[b]{0.25\columnwidth}
		\raisebox{-.5\height}{\includegraphics[width=1.0\linewidth]{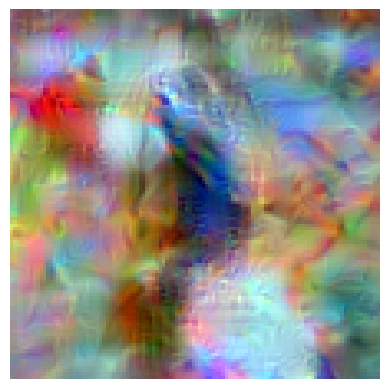}}
	\end{minipage}}  
            & \SetCell[r=1]{l}{\begin{minipage}[b]{0.25\columnwidth}
		\raisebox{-.5\height}{\includegraphics[width=1.0\linewidth]{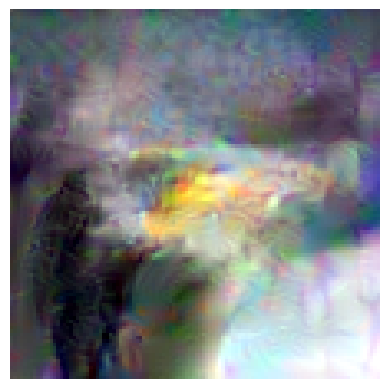}}
	\end{minipage}}  
            & \SetCell[r=1]{l}{\begin{minipage}[b]{0.25\columnwidth}
		\raisebox{-.5\height}{\includegraphics[width=1.0\linewidth]{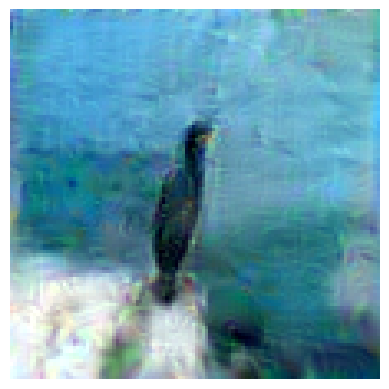}}
	\end{minipage}}                      
            & \SetCell[r=1]{l}{\begin{minipage}[b]{0.25\columnwidth}
		\raisebox{-.5\height}{\includegraphics[width=1.0\linewidth]{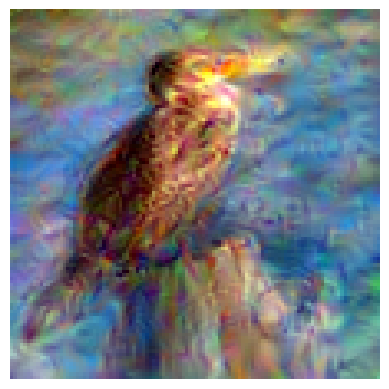}}
	\end{minipage}}  
            & \SetCell[r=1]{l}{\begin{minipage}[b]{0.25\columnwidth}
		\raisebox{-.5\height}{\includegraphics[width=1.0\linewidth]{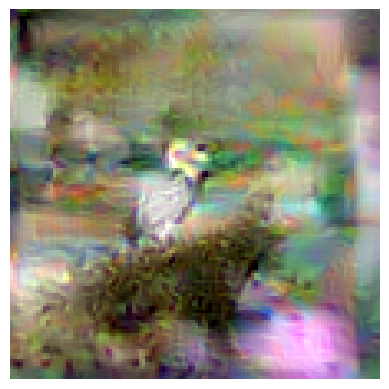}}
	\end{minipage}}  
            & \SetCell[r=1]{l}{\begin{minipage}[b]{0.25\columnwidth}
		\raisebox{-.5\height}{\includegraphics[width=1.0\linewidth]{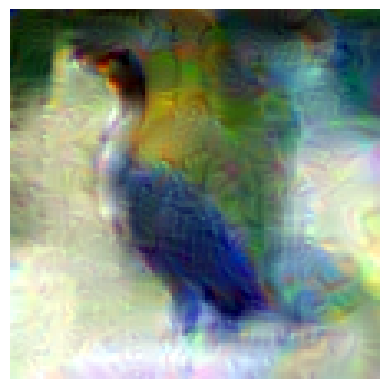}}
	\end{minipage}}
            & \SetCell[r=1]{l}{\begin{minipage}[b]{0.25\columnwidth}
		\raisebox{-.5\height}{\includegraphics[width=1.0\linewidth]{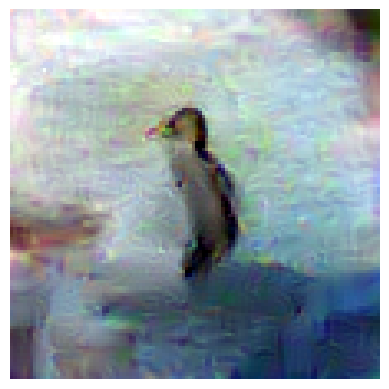}}
	\end{minipage}}
            & \SetCell[r=1]{l}{\begin{minipage}[b]{0.25\columnwidth}
		\raisebox{-.5\height}{\includegraphics[width=1.0\linewidth]{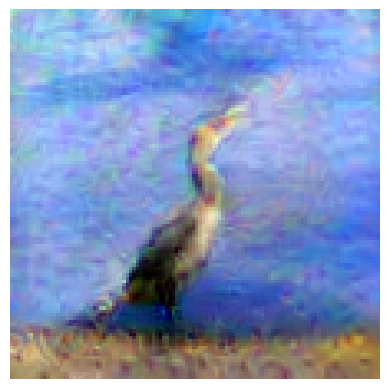}}
	\end{minipage}}
            & \SetCell[r=1]{l}{\begin{minipage}[b]{0.25\columnwidth}
		\raisebox{-.5\height}{\includegraphics[width=1.0\linewidth]{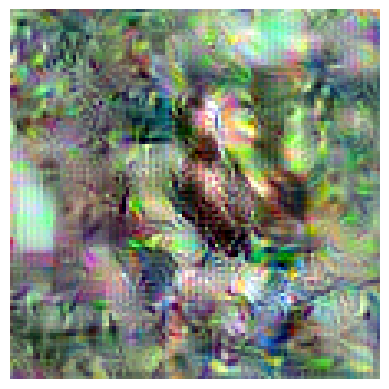}}
	\end{minipage}}
            & \SetCell[r=1]{l}{\begin{minipage}[b]{0.25\columnwidth}
		\raisebox{-.5\height}{\includegraphics[width=1.0\linewidth]{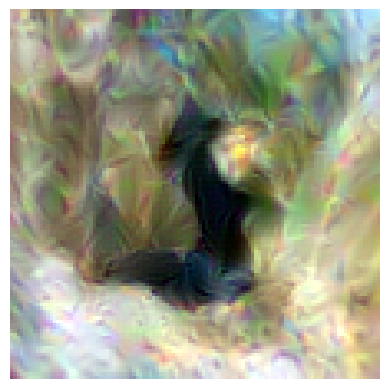}}
	\end{minipage}}     
            \\
PSNR         &8.414&10.661&10.347&11.969&12.119&12.118&12.476&11.205&13.928&9.664&10.358&13.381   \\
LPIPS        &0.474&0.525&0.651&0.61&0.51&0.483&0.534&0.527&0.501&0.441&0.646&0.529    \\
SSIM       &0.243&0.177&0.173&0.343&0.4&0.174&0.217&0.219&0.346&0.297&0.079&0.121
\end{tblr}
}

\caption{CTGI inversion result on CalTech256}
\label{SubTable_appInversionResultSubCal}
\end{subtable}
\end{table*}

\begin{figure*}[h]
    \centering
    \resizebox{\linewidth}{!}{        \includegraphics{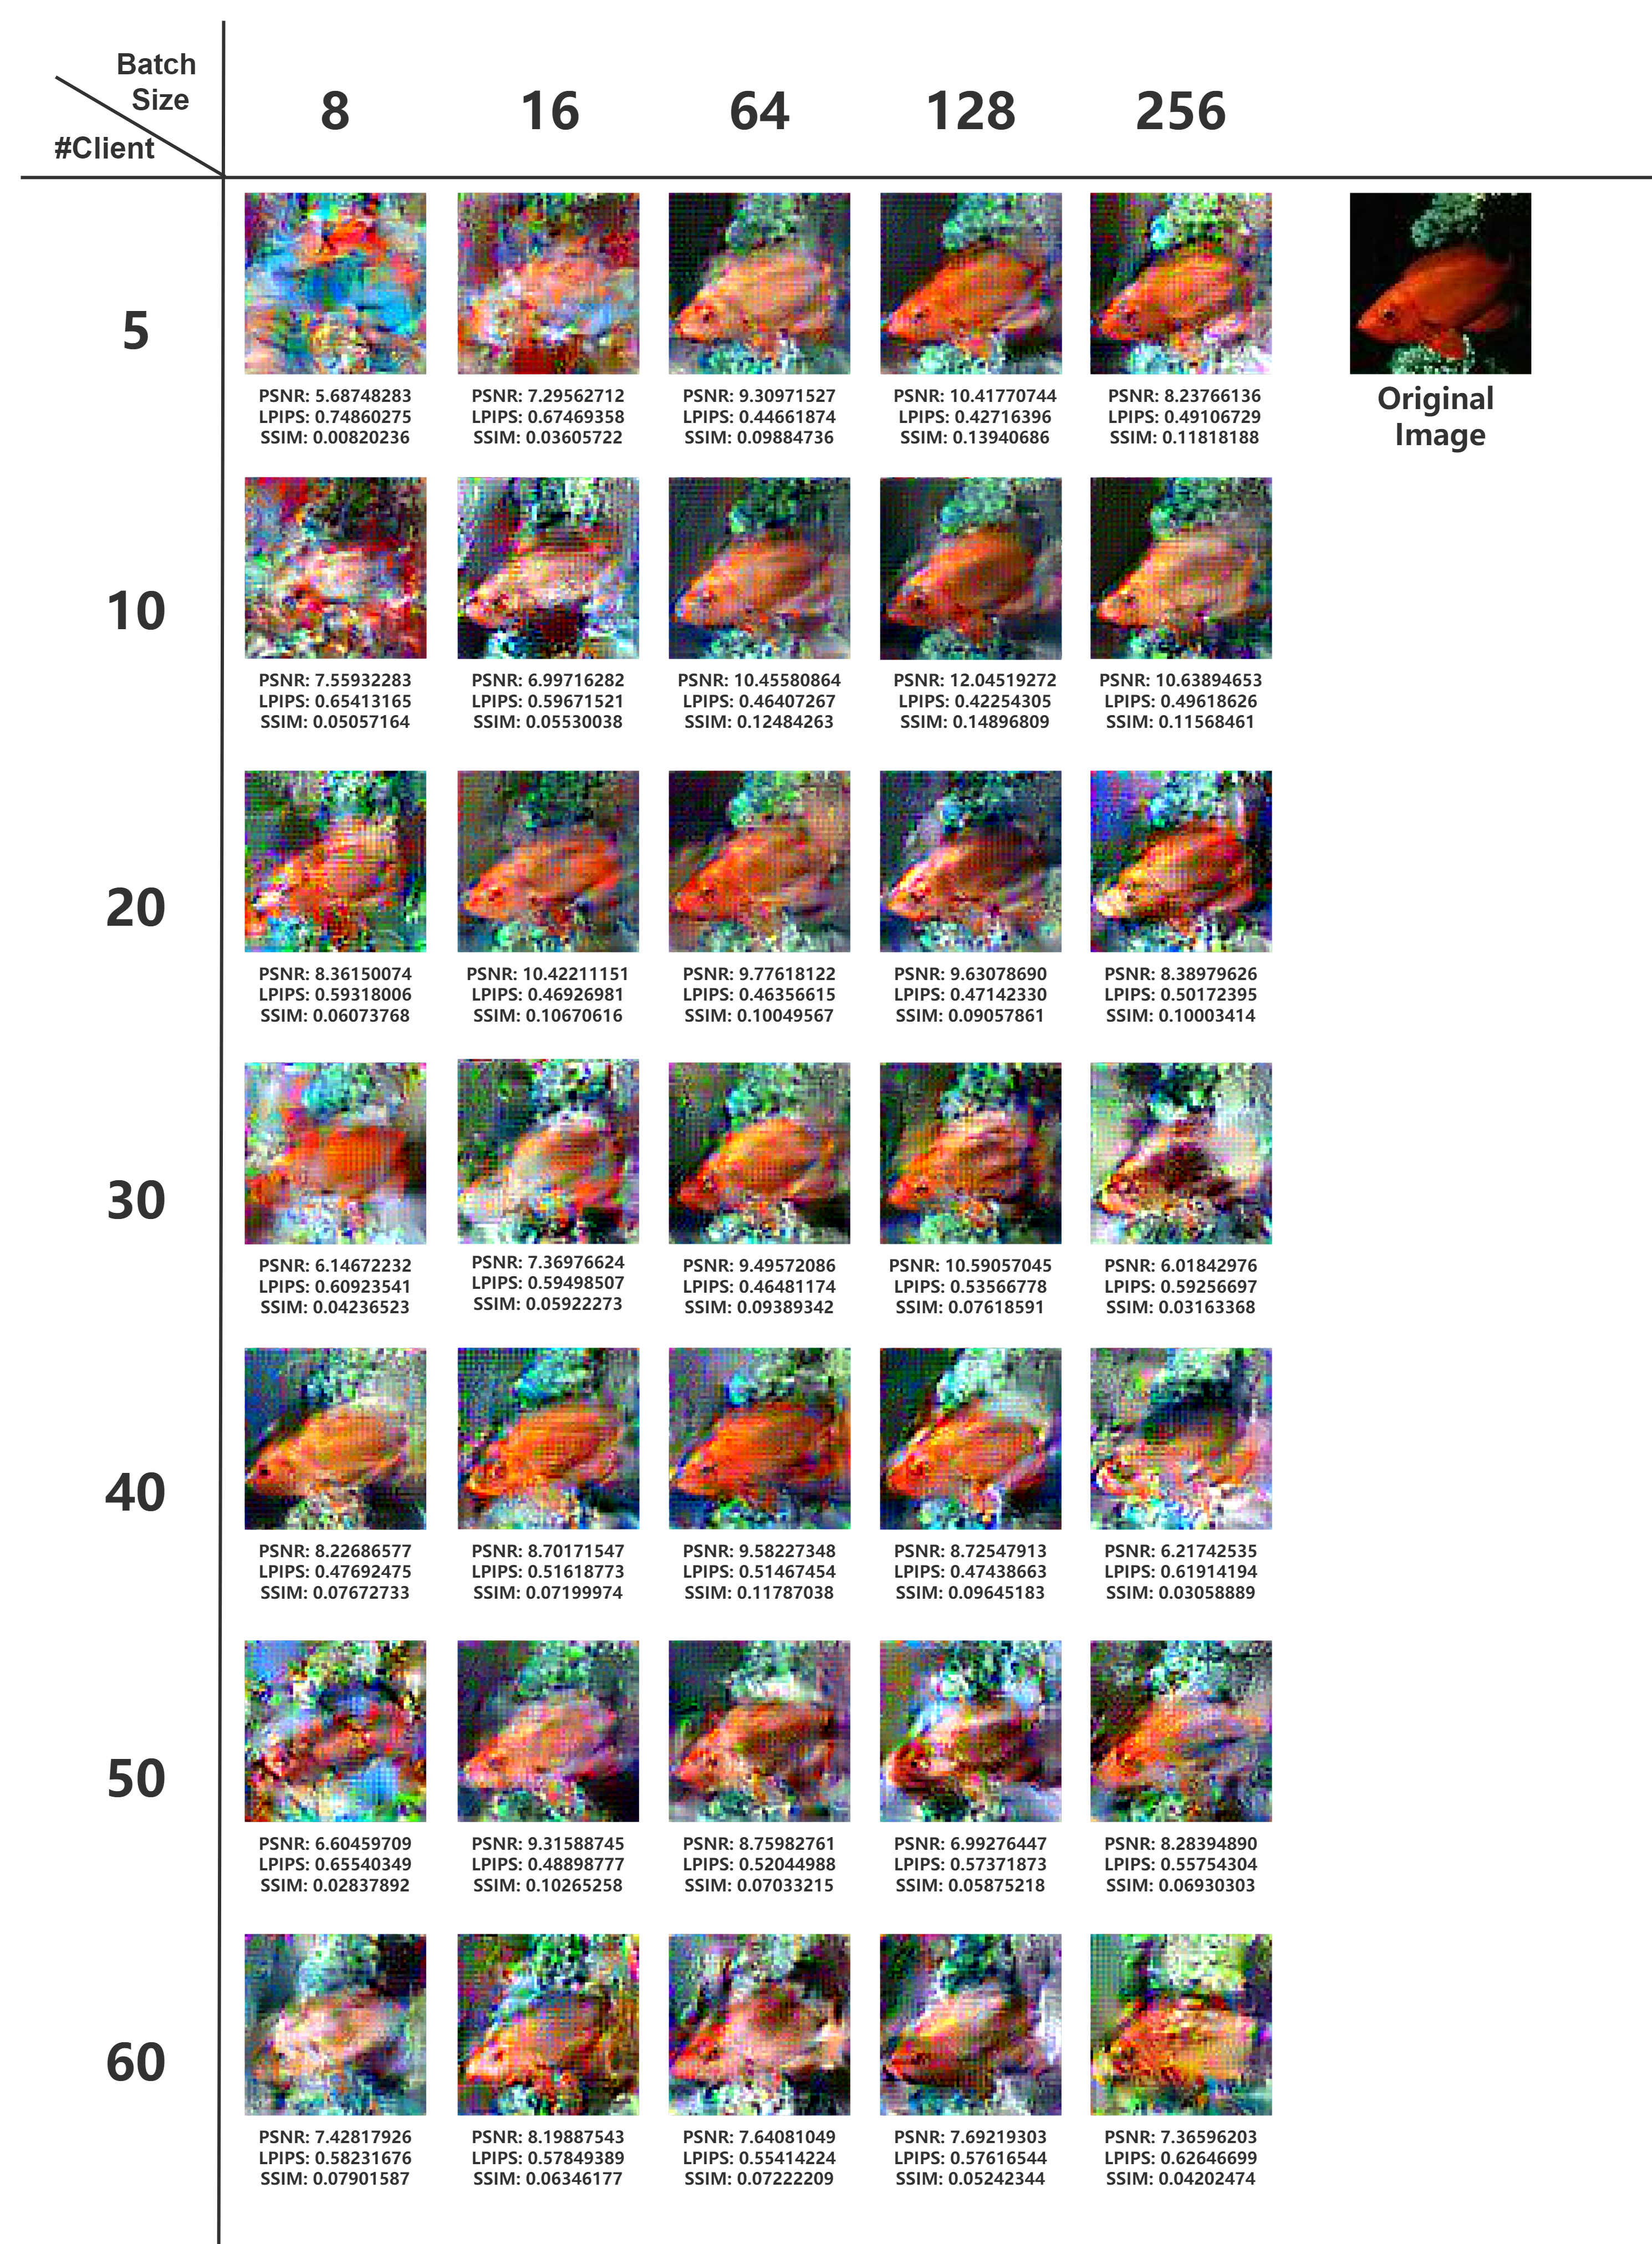}
    }   
    \caption{Inversion Results in exploring the effect of batch size and the number of clients. Detailed information in section \ref{subsection-batch-effect}}
    \label{FigA_BatchEffect}
\end{figure*}
